# Supplementary material for: EADReg: Probabilistic Correspondence Generation with Efficient Autoregressive Diffusion Model for Outdoor Point Cloud Registration
Source: arXiv:2411.15271 source file (2024-11-22)
Supplement: Supplementary file 1 [file X_suppl.tex]

\clearpage
\setcounter{page}{1}
\maketitlesupplementary

\begin{figure*}
\centering
\includegraphics[width=1\textwidth]{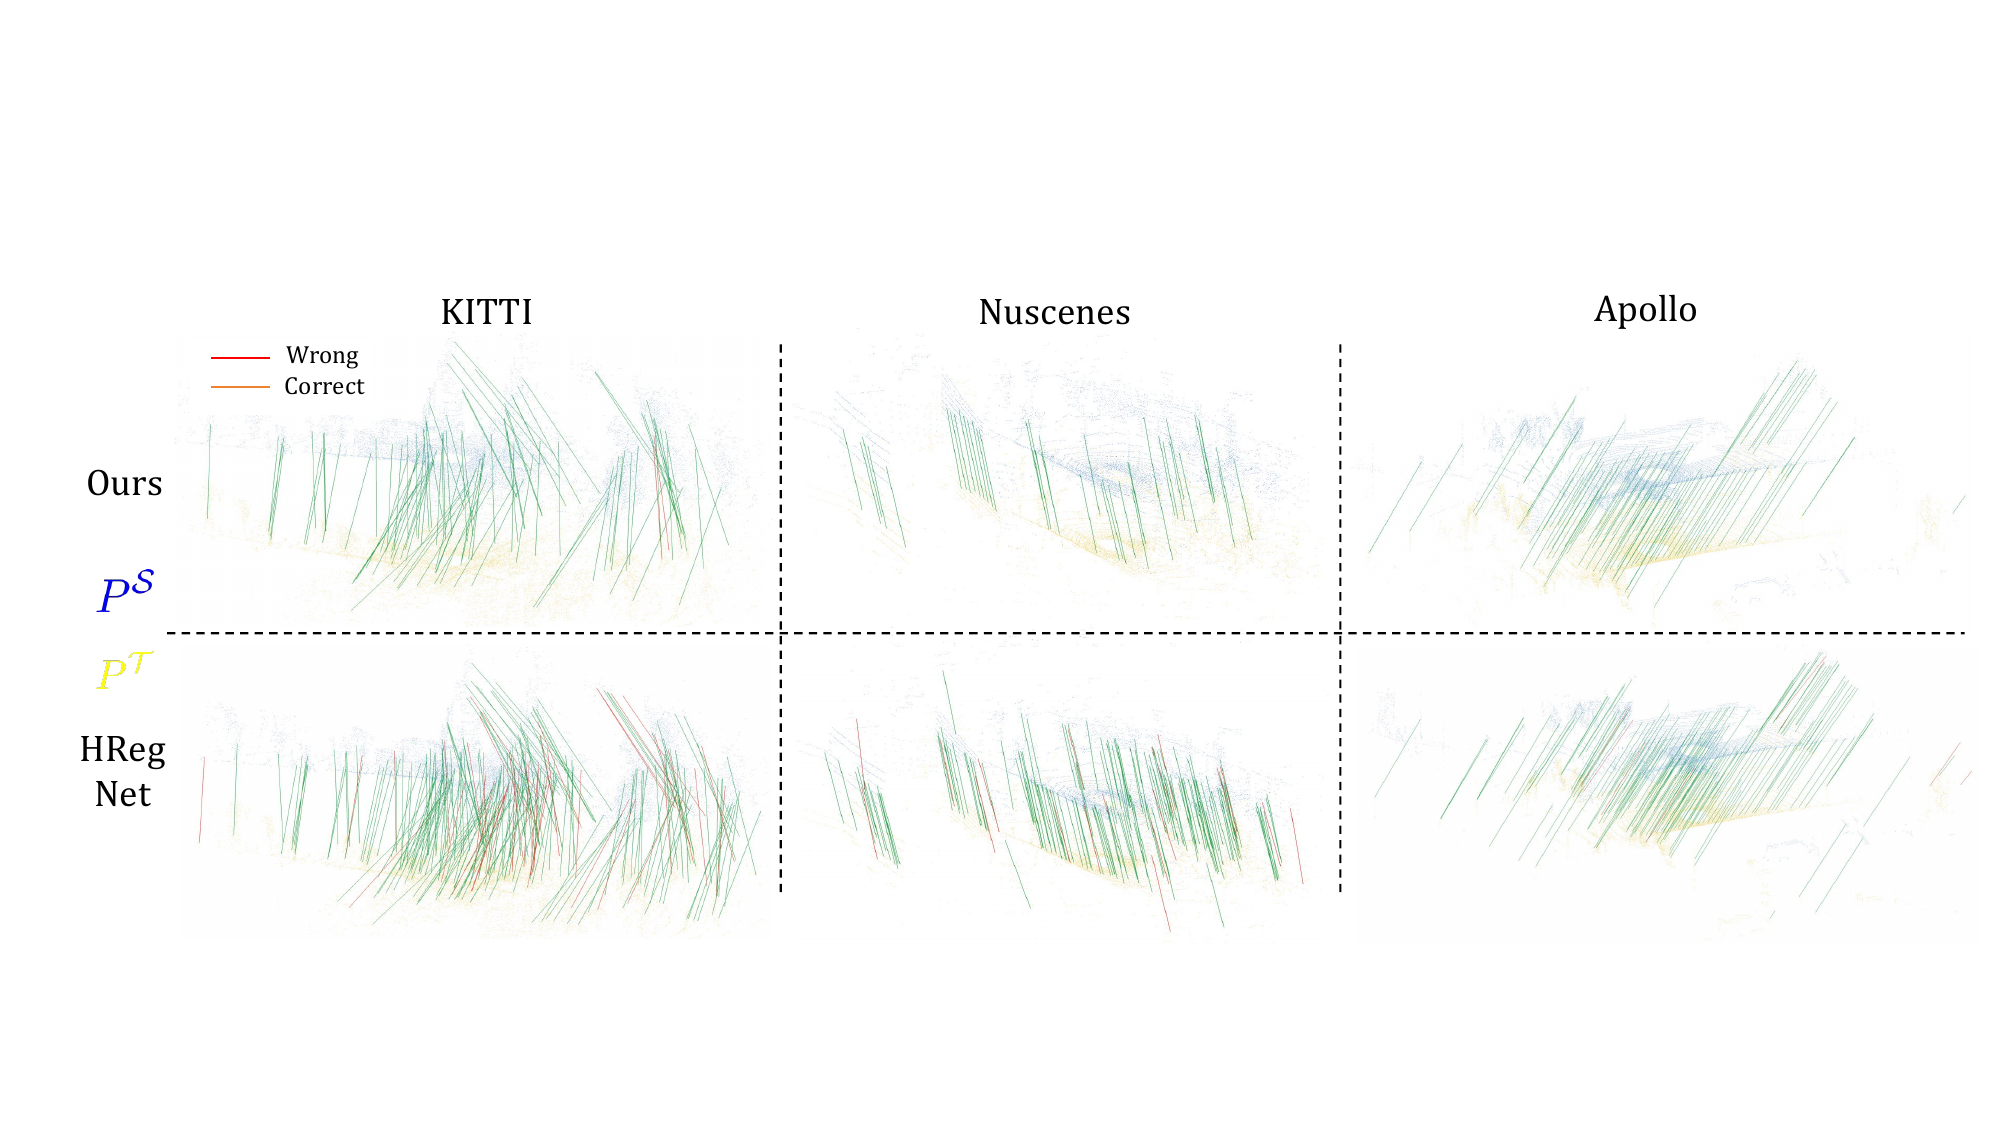}
% \vspace{-0.8cm}
\caption{Qualitative visualization of registration performance. From left to right, we compare our proposed method with HRegNet using three samples from the KITTI, NuScenes, and Apollo-Southbay datasets, respectively. Specifically, we select only the correspondences with confidence weights $\hat{w}$ greater than 0.001.}
\label{fig.correspondence}
	% \vspace{-5mm}

\end{figure*}

\begin{figure*}
\centering
\includegraphics[scale=0.7]{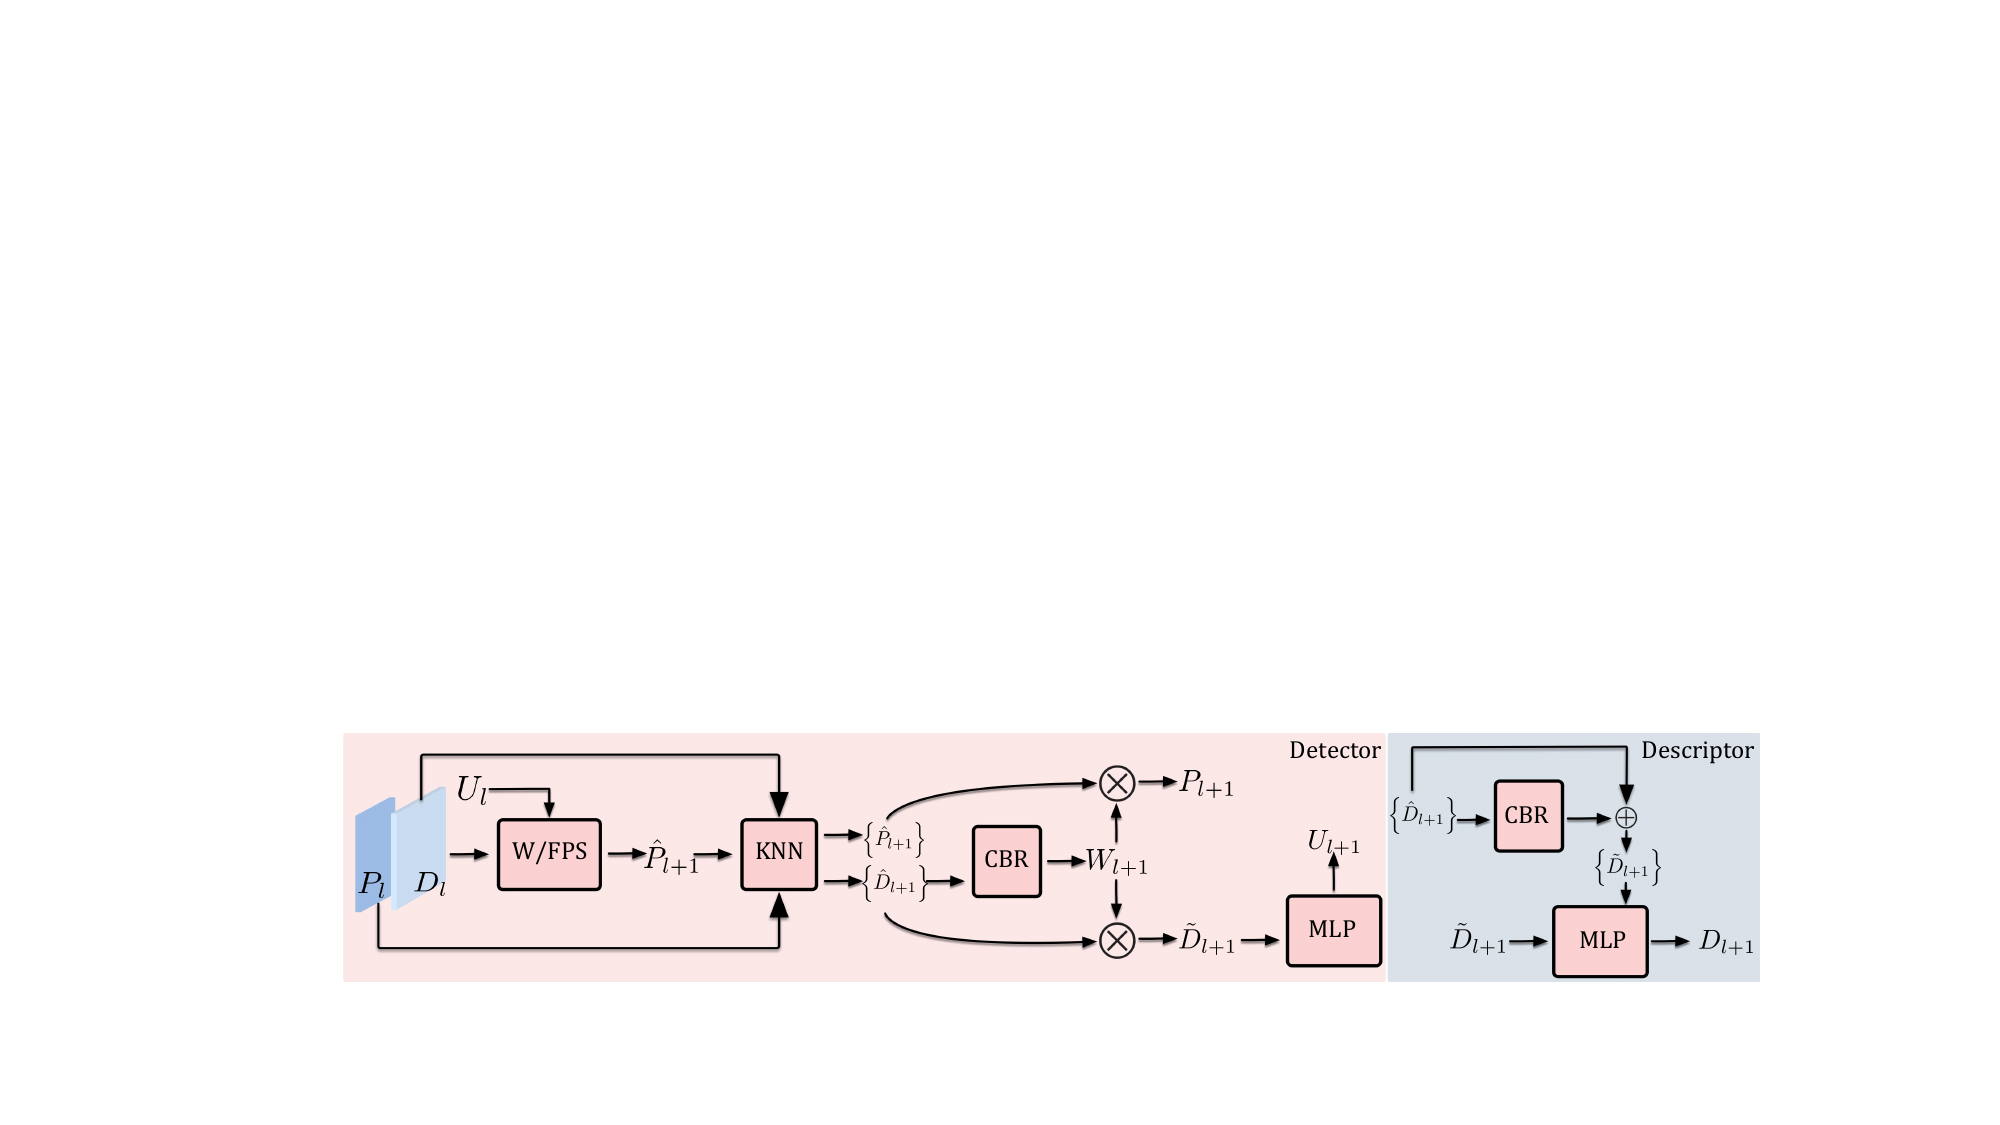}
% \vspace{-0.8cm}
\caption{The backbone of EADReg consists of two main components: the detector and the descriptor. Given the superpoints and their corresponding features as input, the detector uses WFPS (with FPS applied in the first layer) to downsample the input points. By performing KNN searches around each downsampled point in relation to the input points and incorporating CBR modules, the superpoints for the next layer are obtained. The uncertainty values are computed through a MLP module. The detector leverages both the CBR module and MLP layers to generate the features corresponding to the next layer.}
\label{fig.x_backbone}
	% \vspace{-5mm}

\end{figure*}

\begin{figure}
\centering
\includegraphics[scale=0.5]{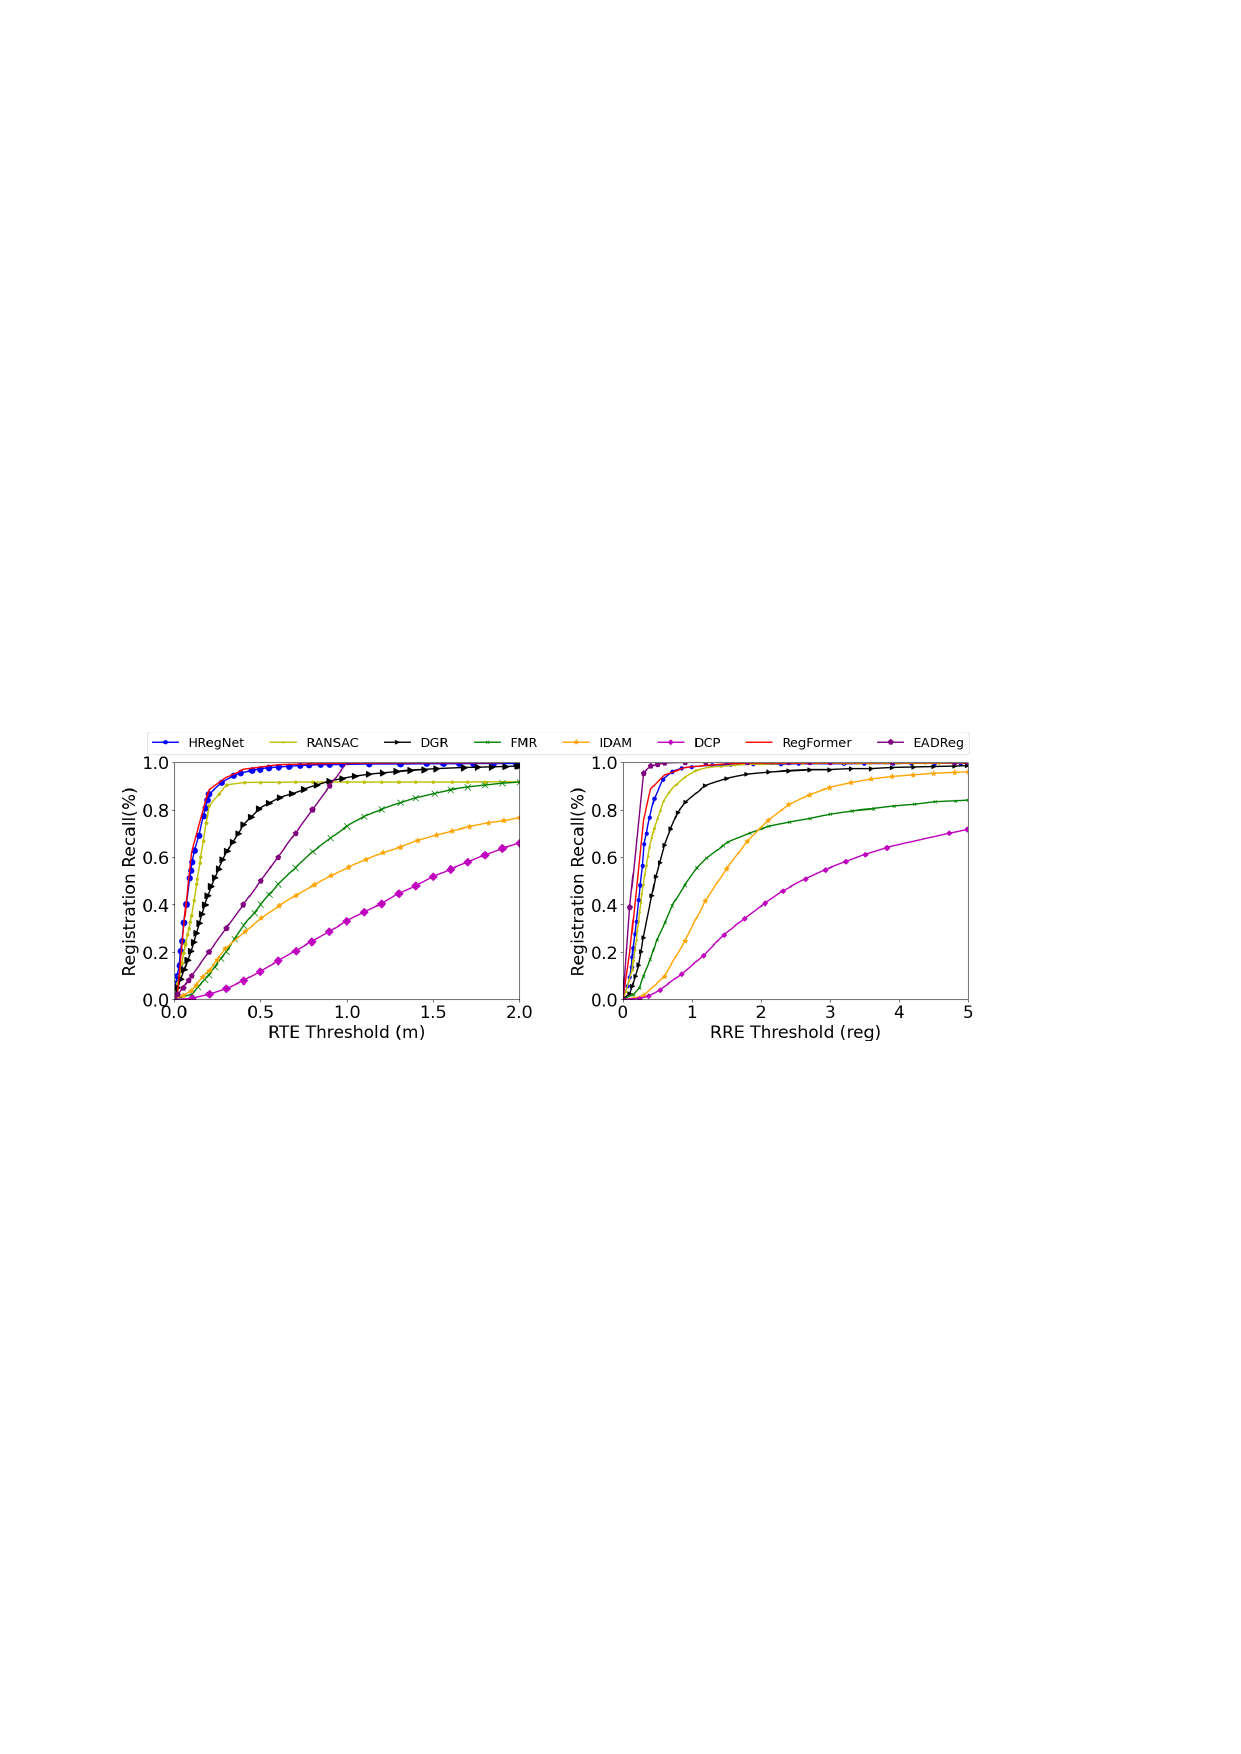}
% \vspace{-0.2cm}
\caption{Registration recall with different RRE and RTE thresholds on the KITTI dataset.}
\label{fig.supple_threshold_}
\end{figure}

\begin{table}[ht]
\centering
	\footnotesize

\caption{Detailed hyperparameters of the detector-descriptor backbone.}
\begin{tabular}{c|c|c|c|c}
        \toprule
\textbf{Layer} & \textbf{$N$} & \textbf{$K$} & \textbf{Detector Convs}       & \textbf{Descriptor Convs}     \\         \midrule

1           &1024        & 64         & $32 \rightarrow 32 \rightarrow 64$  & $32 \rightarrow 32 \rightarrow 64$  \\ 
              \midrule
2              & 512           & 32           & $64 \rightarrow 64 \rightarrow 128$ & $64 \rightarrow 64 \rightarrow 128$ \\ 
              \midrule
3              & 256           & 16           & $128 \rightarrow 128 \rightarrow 256$ & $128 \rightarrow 128 \rightarrow 256$ \\ 
               \bottomrule

\end{tabular}
\label{tab:x_backbone}
\end{table}

\begin{table}[t]
    \centering
% \resizebox{\columnwidth}{!}{%
	\footnotesize
    \caption{Ablation study results of the hyperparameter $\beta$'s influence on the registration results on KITTI dataset. The best results for each criterion are labeled in bold.}

    \begin{tabular}{c|ccc}
        \toprule
                  		$\beta $ & RTE (m) & RRE (deg) & Recall \\

        \midrule
        $\beta =0.5$  & $0.042 \pm 0.043 $&$0.11\pm 0.123$&$ 99.99\%$ \\
        \rowcolor{gray!30}$\beta =1$  &$\mathbf{0.040\pm 0.035}$ & $0.116\pm 0.096$&100\% \\
        $\beta =2$  & $0.041 \pm0.039 $&$0.127\pm0.113$& $100.00\%$  \\
        $\beta =3$  & $0.042 \pm 0.040$ &$0.134\pm0.123$&$ 99.99\% $\\
        \bottomrule
    \end{tabular}
        \label{tab:x_beta}

\end{table}

\begin{table}[t]
    \centering

% \resizebox{\columnwidth}{!}{%
	\footnotesize
    \caption{Ablation study results of the hyperparameter $\gamma$'s influence on the registration results on KITTI dataset. The best results for each criterion are labeled in bold.}

    \begin{tabular}{c|ccc}
        \toprule
                  		$\gamma$ & RTE (m) & RRE (deg) & Recall \\

        \midrule
        $\gamma =0.5$  & $0.041 \pm 0.044 $&$0.123\pm 0.113$&$ 99.81\%$ \\
        \rowcolor{gray!30}$\gamma =1$ &$\mathbf{0.040\pm 0.035}$ & $0.116\pm 0.096$&100\% \\
        $\gamma =2$  &$ 0.041 \pm0.035$ &$0.120\pm0.115$& $100.00\%$  \\
        $\gamma =4$  & $0.041 \pm 0.039$ &$0.121\pm0.120$&$ 99.99\% $\\
        $\gamma =6$  & $0.041 \pm 0.044$ &$0.120\pm0.120$&$ 99.97\% $\\
        \bottomrule
    \end{tabular}
            \label{tab:x_gamma}

\end{table}

\section{Backbone Details}
\label{sec:x_backbone}
The backbone of EADReg, shown in \cref{fig.x_backbone}, comprises two main components: the detector and the descriptor. The input points and their corresponding features are denoted as \( P_l \) and \( D_l \), where the subscript \( l \) represents the layer index (\( l \in \{1, 2, 3\} \)). The detector employs Weighted Farthest Point Sampling (WFPS)\cite{x_detector}, with Farthest Point Sampling (FPS) applied in the first layer, to downsample the input points. WFPS considers the uncertainty of each point, resulting in improved downsampling performance compared to traditional FPS.

By performing K-Nearest Neighbor (KNN) searches around each downsampled point relative to the input points, we obtain the point and descriptor groups \( \{\hat{P}_{l+1}\} \in \mathbb{R}^{N_{l+1} \times K_{l+1} \times 3} \) and \( \{\hat{D}_{l+1}\} \in \mathbb{R}^{N_{l+1} \times K \times d} \), respectively. CBR modules are then employed to compute the weights \( W_{l+1} \) for each group component, enabling the generation of fused points \( P_{l+1} \) and their corresponding features \( D_{l+1} \).  

Uncertainty values are estimated through an MLP module. The detector integrates both CBR modules and MLP layers to produce the features for the subsequent layer. The dimensions of \( K \), the output points, and their corresponding features are detailed in \cref{tab:x_backbone}, where \( \rightarrow \) indicates the dimension changes during forward propagation.

\section{Qualitative Visualization}
\label{sec:x_vis}
Addition to Sec. 4 in our paper, We visualize our proposed EADReg and baseline HRegNet on 3 samples from KITTI, Nuscenes and Apollo datasets in Fig.\ref{fig.correspondence} to evaluate the performance of EADReg.

\section{Quantitative Evaluation}
\label{sec:x_vis}

We present the registration recall rates under various RRE and RTE threshold settings on KITTI dataset in \cref{fig.supple_threshold_}. The results clearly demonstrate that EADReg exhibits superior robustness compared to other methods.

\section{Ablation Study}
\label{sec:x_abs}
The overall loss function in Sec. 3 can be rewritten as: 
\begin{equation}
    \mathcal{L}=\beta \mathcal{L}_\text{trans}+\alpha \mathcal{L}_\text{rot}+ \gamma \mathcal{L}_\text{diff},
\end{equation}
In this section, we will provide the ablation study results of the influence of the hyperparameters $\beta$ and $\gamma$.

\noindent\textbf{Weight of the $\beta$}:
The results in \cref{tab:x_beta} demonstrate that \(\beta = 1\) delivers the best overall registration performance, achieving the lowest RTE and competitive RRE while maintaining a 100\% recall. As \(\beta\) increases, the RTE does not improve, and the RRE gradually degrades, likely due to the decreasing relative weight of \(\alpha \mathcal{L}_\text{rot}\) in the overall loss function. This underscores the importance of maintaining a proper balance between \(\beta \mathcal{L}_\text{trans}\) and \(\alpha \mathcal{L}_\text{rot}\) to optimize registration accuracy. Overemphasizing or underemphasizing either term leads to suboptimal results.

\noindent\textbf{Weight of the ${\gamma}$}:
We present an ablation study on the influence of the hyperparameter \(\gamma\) on the final registration performance in \cref{tab:x_gamma}.  
The results demonstrate that \(\gamma = 1\) delivers the best overall performance, achieving the lowest RTE and RRE errors, along with the most stable variances (\(0.035\) and \(0.096\), respectively). Deviating from this optimal value results in slight degradations in both RTE and RRE. Furthermore, the recall diminishes when \(\gamma\) is either too low (\(0.5\)) or too high (\(6\)), emphasizing the importance of appropriately balancing this parameter.
